# Supplementary material for: On the Effectiveness of Regularization Against Membership Inference Attacks
Source: arXiv:2006.05336 source file (2020-06-09)
Supplement: Supplementary file 1 [file appendix.tex]

\appendix

\section{Membership Inference Attacks}
\label{appendix:mia_details}
\topic{Yeom et al.'s Attack}

\topic{Salem et al.'s Attack}

\section{Mechanisms Against Membership Inference Attacks}
\label{appendix:reg_details}
\topic{Distillation}

\topic{Label Smoothing}

\topic{Adding Gaussian Noise to Training Samples}

\topic{Random Cropping}

\topic{Dropout}

\topic{Spatial Dropout}

\topic{Weight Decay}

\topic{Early Stopping}

\topic{Differential Privacy}
